# Supplementary material for: Learning Visual-Audio Representations for Voice-Controlled Robots
Source: arXiv:2109.02823 source file (2023-03-05)
Supplement: Supplementary file 1 [file Appendix.tex]

\section{Appendix}
\label{sec:append}
Not provided in the submitted version
